# Supplementary material for: Connecting Neural Response measurements & Computational Models of language: a non-comprehensive guide
Source: arXiv:2203.05300 source file (2022-03-10)
Supplement: Supplementary file 1 [file appendix.tex]

\section{List of included color terms}
Red, green, maroon, brown, black, blue, purple, orange, pink, yellow, peach, white, gray, olive, turquoise, violet, lavender, and aqua. 
\label{app:color_terms}

\section{RSA between models}
Figure \ref{fig:rsa_heatmap} shows a the result of representation similarity analysis between the representations derived from all models (and configurations) as well as CIELAB, showing Kendall's correlation coefficient between flattened RSMs.
\label{app:model_rsa}
\begin{figure*}[ht]
\centering
\includegraphics[scale=0.99]{figures/color_rsm.jpeg}
\caption{Result of representation similarity analysis between all models (and configurations), showing Kendall's correlation coefficient between flattened RSMs. Results are shown for layers which are maximally correlated with CIELAB, per model. \texttt{-rc} indicates \textbf{random-context}, \texttt{-cc} indicates \textbf{controlled-context}, and \texttt{-nc} indicates \textbf{non-context}. }
\label{fig:rsa_heatmap}
\end{figure*}

\section{Representation Similarity Matrices}

Figures \ref{fig:cielab_rsm} to \ref{fig:electra_rsm} show the representation similarity matrices employed for the RSA analyses, for the layer with the highest RSA score from each of the controlled-context (CC) models.

\begin{figure*}[ht]
\centering
\includegraphics[scale=0.99]{figures/all_bert_cielab.png}
\caption{CIELAB RSM}
\label{fig:cielab_rsm}
\end{figure*}

\begin{figure*}[ht]
\centering
\includegraphics[scale=0.99]{figures/all_bert_emb.png}
\caption{BERT(CC) RSM}
\label{fig:bert_rsm}
\end{figure*}

\begin{figure*}[ht]
\centering
\includegraphics[scale=0.99]{figures/all_roberta_emb.png}
\caption{RoBERTa(CC) RSM}
\label{fig:roberta_rsm}
\end{figure*}

\begin{figure*}[ht]
\centering
\includegraphics[scale=0.99]{figures/all_google_electra_emb.png}
\caption{ELECTRA(CC) RSM}
\label{fig:electra_rsm}
\end{figure*}

\label{app:rsms}

\section{Warm vs. Cool colors}
\label{app:temp}
Figures \ref{fig:temp_lm} and \ref{fig:temp_rsa} show Linear Mapping and RSA results broken down by color temperature. The color space is split according to temperature measured according to the Hue dimension in the Hue-Value-Saturation space\footnote{\url{https://psychology.wikia.org/wiki/HSV\_color\_space}}.  

\begin{figure*}[ht]
\centering
\includegraphics[scale=0.24]{figures/warm_cool.png}
\caption{Linear mapping results (proportion of explained variance) broken down by color chip temperature for each of the baselines and the LMs.}
\label{fig:temp_lm}
\end{figure*}

\begin{figure*}[ht]
\centering
\includegraphics[scale=0.24]{figures/warm_cool_rsa.png}
\caption{RSA results (Kendall's $\tau$ ) broken down by color temperature for each for each of the baselines and the LMs.}
\label{fig:temp_rsa}
\end{figure*}

\section{Corpus statistics}
Figures \ref{fig:freq} and \ref{fig:entropies} show log frequency and entropy of distributions over part-of-speech categories, dependency relations, and lemmas of dependency tree heads of color terms in common crawl.
 \label{app:corpus_stats}

\begin{figure*}[ht]
\centering
\includegraphics[width=0.6\textwidth]{figures/log_freq.png}
\caption{Log frequency of color terms in common crawl.}
\label{fig:freq}
\end{figure*} 

\begin{figure*}[ht]
\centering
\includegraphics[width=\textwidth]{figures/cc_large_pos_head_and_dep_entropy.png}
\caption{Entropy of distributions over part-of-speech categories, dependency relations, and lemmas of dependency tree heads of color terms in common crawl.}
\label{fig:entropies}
\end{figure*}

%\begin{figure*}[ht]
%\centering
%\includegraphics[width=\textwidth]{figures/cc_large_pos_head_and_dep.png}
%\caption{Log frequency of color terms in common crawl.}
%\label{fig:top}
%\end{figure*} 

\section{Linear mapping results by munsell color chip}
Figure \ref{fig:munsell_full} shows linear mapping results broken down by Munsell chip for all models and configurations.
\label{app:munsell_full}
\begin{figure*}[ht]
\centering
\includegraphics[scale=0.16]{figures/all_munsell_grid_enc.png}
\caption{Linear mapping results for each of the baselines and language models, under all extraction configurations, broken down by Munsell color chip. Each circle on the chart represents the ranking of the predicted color chip when ranked according to Pearson distance ($1 -$ Pearson's $r$) from gold -- the larger the circle, the higher (better) the ranking. Circle colors reflect the modal color term assigned to the chips in the lexicon. Reference plot showing modal color of all chips also included.}
\label{fig:munsell_full}
\end{figure*} 

\section{Linear mapping control task and probe complexity}

\label{app:complexity}
Figure \ref{fig:complexity} shows the full results over a range of probe complexities for the standard experimental condition as well the random control task.

\begin{figure*}[ht]
\centering
         \centering
         \includegraphics[width=\textwidth]{figures/complexity_grid.png}
\caption{Explained variance for the linear probes trained on the normal experimental condition (blue) and the control task (red) where color terms are randomly permuted. The means are indicated by the lines and standard deviation across layers is indicated by the bands.}
\label{fig:complexity}
\end{figure*}

\section{Dimensionality of color subspace}
\label{app:dims}
Figure \ref{fig:dims} shows the proportion of explained variance with respect to the number of dimensions which are assigned $95\%$ of the linear regression coefficient weights. 

\begin{figure*}[ht]
\centering
         \centering
         \includegraphics[width=\textwidth]{figures/rank_grid.png}
\caption{The y-axis shows explained variance for the linear probes. The means are indicated by the lines and standard deviation across layers is indicated by the bands. The x-axis shows the number of regression matrix coefficients assigned $95\%$ of the weight.}
\label{fig:dims}
\end{figure*}

\section{Effect of model size}
\label{app:smaller}
Table \ref{tab:small_results} shows the RSA and linear mapping (selectivity) results for four BERT models: BERT-mini (4 layers, hidden size: 256), BERT-small (4 layers, hidden size: 512), BERT-medium (8 layers, hidden size: 512), and BERT-base (12 layers, hidden size: 768). Model specification and training details for the first three can be found in \newcite{turc2019well} and for last in \newcite{devlin-etal-2019-bert}. 

\begin{table*}[ht]
    \centering
    \footnotesize
     %\resizebox{\pagewidth}{!}{%
    \begin{tabular}{ccc|cc}
        \toprule
        Model & RSA max & RSA mean & lin. map.. max & lin. map. mean \\
                \midrule
        BERT-mini & 0.077  & 0.043 $\pm$ 0.340 & 0.729 & 0.582 $\pm$ 0.291 \\
        BERT-small & 0.106  & 0.070 $\pm$ 0.191 & 0.734 & 0.598 $\pm$ 0.294 \\
        BERT-medium & 0.097  & 0.057 $\pm$ 0.035 & 0.739 & 0.654 $\pm$ 0.221 \\
        BERT-base & 0.162$^{*}$  & 0.092 $\pm$ 0.058 & 0.740 & 0.677 $\pm$ 0.182 \\

        \bottomrule
        
    \end{tabular}
   % }
    \caption{Results for the four smaller BERT models. RSA results (left) show max and mean (across layers) Kendall's correlation coefficient ($\tau$). Correlations that are significantly non-zero are indicated with: * : $p < 0.05$.  Results for the Linear Mapping experiments (right) show max and mean selectivity. Standard deviation across layers is included with the mean results.}
    \label{tab:small_results}
\end{table*}

\section{Linear Mixed Effects Model}
\label{app:lme}
To fit Linear Mixed Effects Models, we use the \textsc{LME4} package. With model type (BERT-CC, RoBERTa-NC, etc.) as a random effect, we follow a step-wise model construction sequence which proceeds along four levels of nesting: (i) in the first level color log-frequency is the only fixed effect, (ii) in the second \texttt{pmi-colloc} is added to that, (iii) in the third, each of \texttt{pos-ent, deprel-ent, head-ent} is added separately to the a model with log frequency and \texttt{pmi-colloc}, (iv) the term that leads to the best fit from the previous level \texttt{deprel-ent} is included, then each of the proportion terms \texttt{adj-prop, amod-prop, cop-prop} is added. The reported regression coefficients are extracted from the minimal model containing each term.
